# Supplementary material for: Structure--property relationships of cell clusters in biotissues: 2D analysis
Source: arXiv:1702.02145 source file (2017-02-07)
Supplement: Supplementary file 1 [file Supplementary_Material.pdf]

Supplementary Material for "Structure–property relationships of cell clusters in biotissues: 2D analysis"

Xiaohua Zhou, Erhu Zhang, Minggang Xia, Jianlin Liu and Shengli Zhang

**S.1. Bead-like structure**

Here we show a bead-like structure composed by three cells adhere together. This model needs to run on the Surface Evolver 2.70s.

```
// Surface Evolver code for bead-like structure composed by three cells.
SPACE_DIMENSION 2
STRING

PARAMETER ad = -4            // ad is the adhesion potential
PARAMETER inputrv = 0.9    // inputrv is the reduced volume

VIEW_MATRIX
      1.000000000000000     0.000000000000000    -0.952000000000001
      0.000000000000000     1.000000000000000    -0.700000000000000
      0.000000000000000     0.000000000000000     1.000000000000000

define edge attribute sqcurve_string_mark integer
QUANTITY sqc_c1 ENERGY method sqcurve_string_marked global modulus 0.5 parameter_2 1
QUANTITY sqc_c2 ENERGY method sqcurve_string_marked global modulus 0.5 parameter_2 2
QUANTITY sqc_c3 ENERGY method sqcurve_string_marked global modulus 0.5 parameter_2 4
QUANTITY c1_length FIXED = 2*Pi method edge_length
QUANTITY c2_length FIXED = 2*Pi method edge_length
QUANTITY c3_length FIXED = 2*Pi method edge_length

vertices          /*   coordinates   */
1    0      0
2    1      0
3    0      1
4    1      1
5    0      2
6    1      2
7    0      3
8    1      3

edges
1    1    2   tension 0      sqcurve_string_mark 1      QUANTITY c1_length                              color blue
2    2    4   tension 0      sqcurve_string_mark 1      QUANTITY c1_length                              color blue
3    4    3   tension ad/2   sqcurve_string_mark 1+2    QUANTITY c1_length QUANTITY c2_length color red
4    3    1   tension 0      sqcurve_string_mark 1      QUANTITY c1_length                              color blue
5    4    6   tension 0      sqcurve_string_mark 2      QUANTITY c2_length                              color blue
6    6    5   tension ad/2   sqcurve_string_mark 2+4    QUANTITY c2_length QUANTITY c3_length color red
7    5    3   tension 0      sqcurve_string_mark 2      QUANTITY c2_length                              color blue
8    6    8   tension 0      sqcurve_string_mark 4      QUANTITY c3_length                              color blue
9    8    7   tension 0      sqcurve_string_mark 4      QUANTITY c3_length                              color blue
10   7    5   tension 0      sqcurve_string_mark 4      QUANTITY c3_length                              color blue

faces      /* edge loop */
1      1      2    3      4
2     -3      5    6      7
3     -6      8    9      10
bodies   /* facets */
1      1
2      2
3      3

read
setad:= {set edge tension ad/2 where color == 4 }
```

```
setrv:= { set body[1] target (inputrv*pi); set body[2] target (inputrv*pi); set body[3] target (inputrv*pi); }
suml := { La := sum(edges where color == 4,length);
          La12 := sum(edges where original == 3,length);
          La23 := sum(edges where original == 6,length)}
report := { suml; rvt1 := body[1].volume/pi; rvt2 := body[2].volume/pi; rvt3 := body[3].volume/pi;
            Ef := sqc_c1.value + sqc_c2.value + sqc_c3.value;
            Et1 := sqc_c1.value + La12*ad/2;
            Et2 := sqc_c2.value + La12*ad/2 + La23*ad/2;
            Et3 := sqc_c3.value + La23*ad/2 ;
            Ea:= ad*La; Et := Ef + ad*La;
            printf "adhesion potential is %f, total adhesion length is %f, total energy is %f", ad, La, Et}
c1 := { { g 10; V } 100}
c2 := {r; r; r; {c1}10; r; {c1}10}
c3 := {r; r; r; {c1}10;setrv; {c1}10; r; {c1}10}
// Using the c3 or c2 order, we can obtain the structure with or without volume constraint.
```

**S.2. Periodic square structure**

Here we show a periodic square structure model which needs to run on the Surface Evolver 2.70s.

```
// Surface Evolver code for periodic square structure.
SPACE_DIMENSION 2
STRING
LINEAR
PARAMETER ad =    -4
PARAMETER RDx =    1.8    // period length on x direction
PARAMETER RDy =    1.8    // period length on y direction
PARAMETER inputrv = 0.94
PARAMETER RR = 1/4*(RDx+RDy)/cos(pi/8)

torus
periods
RDx    0
0    RDy

view_matrix
  1.0    0      3.65
  0      1.0    1.85
  0       0       1

define edge attribute sqcurve_string_mark integer
quantity sqc1 energy method sqcurve_string_marked modulus 0.5 global parameter_2 1
quantity sqc2 energy method sqcurve_string_marked modulus 0.5 global parameter_2 2
quantity sqc3 energy method sqcurve_string_marked modulus 0.5 global parameter_2 4
quantity sqc4 energy method sqcurve_string_marked modulus -0.5 global parameter_2 8
method_instance ves_length_1 method edge_length modulus 1
method_instance ves_length_2 method edge_length modulus 2
quantity ves_length fixed = 2*pi method ves_length_1 method ves_length_2

vertices
   1    RR*cos(-5*pi/24)-RDx          RR*sin(-5*pi/24)
   2    RR*cos(-pi/8)-RDx             RR*sin(-pi/8)
   3    RR*cos(pi/8)-RDx              RR*sin(pi/8)
   4    RR*cos(5*pi/24)-RDx           RR*sin(5*pi/24)
   5    RR*cos(19*pi/24)              RR*sin(19*pi/24)
   6    RR*cos(29*pi/24)              RR*sin(29*pi/24)
   7    RR*cos(7*pi/24)               RR*sin(7*pi/24)-RDy
   8    RR*cos(3*pi/8)                RR*sin(3*pi/8)-RDy
   9    RR*cos(5*pi/8)                RR*sin(5*pi/8)-RDy
   10 RR*cos(17*pi/24)                RR*sin(17*pi/24)-RDy
   11 RR*cos(31*pi/24)                RR*sin(31*pi/24)
   12 RR*cos(41*pi/24)                RR*sin(41*pi/24)

edges
   1        1    2     * *      tension 0          color blue        sqcurve_string_mark 1        ves_length_1
   2        2    3     * *      tension ad/2       color red         sqcurve_string_mark 1+2    ves_length_2
   3        3    4     * *      tension 0          color blue        sqcurve_string_mark 1        ves_length_1
   4        6    2     * *      tension 0          color blue        sqcurve_string_mark 2        ves_length_1
```

```
    5      3    5    * *    tension 0       color blue    sqcurve_string_mark 2       ves_length_1
    6      7    8    * *    tension 0       color blue    sqcurve_string_mark 4       ves_length_1
    7      8    9    * *    tension ad/2    color red     sqcurve_string_mark 2+4     ves_length_2
    8      9    10   * *    tension 0       color blue    sqcurve_string_mark 4       ves_length_1
    9      12   8    * *    tension 0       color blue    sqcurve_string_mark 2       ves_length_1
    10     9    11   * *    tension 0       color blue    sqcurve_string_mark 2       ves_length_1
    11     4    7    - +    tension 0       color blue    sqcurve_string_mark 1+4+8   ves_length_1
    12     5    10   * +    tension 0       color blue    sqcurve_string_mark 2+4+8   ves_length_1
    13     6    11   * *    tension 0       color blue    sqcurve_string_mark 2       ves_length_1
    14     12   1    + *    tension 0       color blue    sqcurve_string_mark 1+2+8   ves_length_1

faces      /* edge loop */
    1    1 2 3 11 6 7 8 -12 -5 -2 -4 13 -10 -7-9 14

bodies   /* facets */
    1        1

read
setrv := { set body[1] target (inputrv * pi)}
setad := { set edge tension ad/2 where color == 4}
suml := { La := 2*sum(edges where color == 4,length); Lf := sum(edges where color == 1,length)}
report := { suml;
    rvt := body[1].volume/pi;
    Ef := sqc1.value + sqc2.value+ sqc3.value+ sqc4.value;
    Ea := ad*La/2;
    Et := Ef + Ea;
    printf "ad is %f, La is %f, Lf is %f, Ef is %f, Et is %f, rv is %f", ad,    La, Lf, Ef, Et, rvt}
tran2 := { transform_expr "ab"; show_trans "R"; } // twice in each direction
tran3 := { transform_expr "abab"; show_trans "R"; } // three times in each direction
tran4 := { transform_expr "ababab"; show_trans "R"; } // four times in each direction
tran8 := { transform_expr "7(ab)"; show_trans "R"; } // four times in each direction
tran1 := { transform_expr ""; show_trans "R"; } // just the original
c1 := {{g 10; V }200}
c2 := {g;r;{c1}100;r;{c1}100;tran4}
c3 := {g;r;c1;r;setrv;{c1}100;{c1}100;tran4}
//Using the c3 or c2 order we can obtain periodic square structure with or without volume constraint.
//Using the c2 order, we can see that the adhesion regions are straight lines when there is not volume constraint.
```
